# Supplementary material for: Geo-Llama: Leveraging LLMs for Human Mobility Trajectory Generation with Spatiotemporal Constraints
Source: arXiv:2408.13918 source file (2025-04-28)
Supplement: Supplementary file 1 [file 6.appendix.tex]

% \newpage
\section*{Appendix}
